# Supplementary material for: FedEval: A Holistic Evaluation Framework for Federated Learning
Source: arXiv:2011.09655 source file (2022-12-25)
Supplement: Supplementary file 1 [file appendices.tex]

\section*{Appendix B: Datasets and Parameters} \label{appendix:datasets and parameters}

Following previous work \citep{mcmahan2016communication}, we use $B$, $C$, and $E$ as the parameters of FL mechanisms, $B$ is the local batch size, $C$ is the ratio of clients that participate in each round of training, and $E$ is the number of local training passes (i.e., number of epochs).

\begin{table}
	\centering
	
	\setlength{\tabcolsep}{0.3em}
	\caption{Finetuned Hyperparameters}
	\label{tab:dataset}
	\begin{tabular}{ccccc}
		\toprule
		Dataset & \#Device & \#Sample & Model & Parameters \\
		\midrule
		\tabincell{c}{MNIST \\ \citep{lecun1998gradient}} & 100 & 300 & \tabincell{c}{2-layer \\ MLP} & \tabincell{c}{(FedSGD, FedSTC)$\leftarrow$LR=0.5 \\ (FedAvg, FedProx, FedOpt)$\leftarrow$B=16,LR=0.1} \\ \midrule
		\tabincell{c}{FEMNIST \\ \citep{caldas2018leaf}} & 100 & 137 & LeNet & \tabincell{c}{(FedSGD, FedSTC)$\leftarrow$LR=0.1 \\ (FedAvg, FedProx, FedOpt)$\leftarrow$B=8,LR=0.05}  \\ \midrule
		\tabincell{c}{CelebA \\ \citep{caldas2018leaf}} & 100 & 24 & LeNet & \tabincell{c}{(FedSGD, FedSTC)$\leftarrow$LR=0.1 \\ (FedAvg, FedProx, FedOpt)$\leftarrow$B=4,LR=0.05} \\ \midrule
		\tabincell{c}{Sent140 \\ \citep{go2009twitter}} & 100 & 140 & \tabincell{c}{2-layer \\ LSTM} & \tabincell{c}{(FedSGD, FedSTC)$\leftarrow$LR=0.05 \\ (FedAvg, FedProx, FedOpt)$\leftarrow$B=4,LR=0.0001} \\
		\bottomrule
	\end{tabular}
\end{table}

\Cref{tab:dataset} shows the four benchmarking datasets that we used in the experiments, and the corresponding finetuned parameters. We use 100 clients in all the experiments. We set $B=\infty,C=1$, and $E=1$ for FedSGD, empirically chose B and E for FdAvg, then perform a fine-grained search on learning rates from $0.0001 \sim 1.0$. The best hyperparameters are shown in \Cref{tab:dataset}. The parameter-searching results (e.g., tuning learning rates) are presented in the appendix \ref{appendix:params_tune}. For datasets that are not collected in FL style (e.g., MNIST), we simulate the non-IID data by restricting the number of clients' local image classes. For example, The experiments of clients have 1 class of MNIST images are reported in robustness benchmarks. For datasets collected in FL manner (i.e., the samples are organized by who generated them), we partition the data naturally based on the identity and randomly shuffle the data between clients to create an ideal IID data setting. To simplify the comparison, we only present the non-IID data results in the robustness evaluation and use the IID setting in other experiments.

All the experiments run on a Linux server \highlight{with Ubuntu 18.04 installed, Intel(R) i7-9700KF} 8-core 3.7GHz CPU, 128GB RAM, \highlight{960G SSD storage}. \highlight{All the experiments are performed using FedEval (\url{https://github.com/Di-Chai/FedEval}), which is a benchmarking system maintained by us. All the parties are simulated using docker containers, which are connected using docker network using the bridge mode.} We limit the clients' bandwidth to 100Mb/s and do not restrict the server's bandwidth. We set the network latency to 50ms. \highlight{The reproduction guideline is provided at \url{https://di-chai.github.io/FedEval/Reproduce.html}, and the benchmarking results are also available online at \url{https://di-chai.github.io/FedEval/BenchmarkResults.html}}.
